# Supplementary material for: The sound of an axon's growth
Source: arXiv:1807.04799 source file (2019-04-17)
Supplement: Supplementary file 1 [file Folzetal_SM.pdf]

# Can you hear an axon growing? - Supplementary Material

Frederic Folz, Lukas Wettmann, and Giovanna Morigi
*Theoretische Physik, Universität des Saarlandes, 66041 Saarbrücken, Germany*

Karsten Kruse
*NCCR Chemical Biology, Departments of Biochemistry and Theoretical Physics, University of Geneva, 1211 Geneva, Switzerland*

## LINEAR STABILITY ANALYSIS

We perform a linear stability analysis of Eqs. (5) and (6) similar to [24]. First, we assume $J_0 = J_I = J_O = J$, $\gamma_I = \gamma_O = \gamma$ and introduce $\tilde{c}_I = c_I/\kappa$ and $\tilde{c}_O = c_O/\kappa$. Thus,

$$\dot{\tilde{c}}_I(t) = \frac{J}{\kappa} - \gamma\tilde{c}_I(t) - \frac{J}{\kappa} f_1\left(\tilde{c}_O(t-\tau)\right) \tag{S1}$$

$$\dot{\tilde{c}}_O(t) = -\gamma\tilde{c}_O(t) + \frac{J}{\kappa} f_1\left(\tilde{c}_I(t-\tau)\right) \tag{S2}$$

Let $\tilde{c}_I^*$ and $\tilde{c}_O^*$ denote steady state solutions of Eqs. (S1) and (S2). In the oscillatory regime $\tilde{c}_j^* = \lim_{t\to\infty}\langle\tilde{c}_j(t)\rangle = \lim_{t\to\infty} 1/T\int_t^{t+T} dt'\tilde{c}_j(t')$ (with $j = I, O$). Then, we can write

$$0 = \frac{J}{\kappa} - \gamma\tilde{c}_I^* - \frac{J}{\kappa}\langle f_1(\tilde{c}_O)\rangle\,, \tag{S3}$$

$$0 = -\gamma\tilde{c}_O^* + \frac{J}{\kappa}\langle f_1(\tilde{c}_I)\rangle\,. \tag{S4}$$

In detail, at the instability point it holds $\langle f_1(\tilde{c}_j)\rangle = f_1(\tilde{c}_j^*)$ (with $j = I, O$). We assume small fluctuations about the steady state values and make a Taylor expansion of $f(\tilde{c}_j)$ around $\tilde{c}_j^*$ to first order, which yields

$$f(\tilde{c}_j) \approx f(\tilde{c}_j^*) + f'(\tilde{c}_j^*)y_j\,, \tag{S5}$$

where we introduced $y_j = \tilde{c}_j - \tilde{c}_j^*$. By plugging this expression into Eqs. (S1) and (S2), using Eqs. (S3) and (S4), we get

$$\dot{y}_I(t) = -\gamma y_I(t) - \frac{J}{\kappa} f_1'\left(\tilde{c}_O^*\right) y_O(t-\tau) \tag{S6}$$

$$\dot{y}_O(t) = -\gamma y_O(t) + \frac{J}{\kappa} f_1'\left(\tilde{c}_I^*\right) y_I(t-\tau). \tag{S7}$$

To solve this set of delay differential equations, we make the ansatz $y_j(t) = Y_j e^{\lambda t}$ with $\lambda \in \mathbb{C}$ and $j = I, O$. This leads to the set of equations

$$\underbrace{\begin{pmatrix} (\lambda+\gamma)e^{\lambda\tau} & f'(\tilde{c}_O^*)J/\kappa \\ -f'(\tilde{c}_I^*)J/\kappa & (\lambda+\gamma)e^{\lambda\tau} \end{pmatrix}}_{A:=} \begin{pmatrix} Y_I \\ Y_O \end{pmatrix} = \begin{pmatrix} 0 \\ 0 \end{pmatrix} \tag{S8}$$

This set of equations has a non-trivial solution if the determinant of matrix $A$ vanishes. In this case, we get

$$\lambda = \pm i(J/\kappa)\sqrt{f'(\tilde{c}_I^*)f'(\tilde{c}_O^*)}e^{-\lambda\tau} - \gamma. \tag{S9}$$

In order to find the conditions for a Hopf-bifurcation, we set $\lambda = i\omega$ which yields

$$\tilde{J}\sqrt{f'(\tilde{c}_I^*)f'(\tilde{c}_O^*)}\sin(\omega\tau) = \pm 1 \tag{S10}$$

$$\tilde{J}\sqrt{f'(\tilde{c}_I^*)f'(\tilde{c}_O^*)}\cos(\omega\tau) = \pm\omega/\gamma, \tag{S11}$$

with $\tilde{J} = J/\kappa\gamma$. These equations can be cast into the useful form

$$\cot(\omega\tau) = \omega/\gamma\,, \tag{S12}$$

$$\omega = \pm\gamma\sqrt{\tilde{J}^2 f'(\tilde{c}_I^*)f'(\tilde{c}_O^*) - 1}\,. \tag{S13}$$

In the main text for simplicity we restrict to positive frequencies $\omega$, since the sign of the frequencies is irrelevant for the discussion on the minimal length.

## CHANGES OF THE AXON LENGTH UPON CHANGES OF THE DYNEIN CONCENTRATION

Similarly to the effects of reducing the concentration of kinesin motors, it has been observed that the axon length increases if the dynein concentration is reduced. In our model, we can capture this effect by reducing the coupling parameter $J_O$, which determines the number of motors moving from the growth cone to the soma in response to the incoming signal $I$. As in the experiments, we also find in this case an increase of the axon length, see Fig. S1.

## STOCHASTIC DELAY

In this section we shortly discuss the effect of noise on the delay time $\tau$ on the stability of the solutions. In fact, since the velocity of both Kinesin and Dynein motors follows a statistical distribution, the delay $\tau = L/v$ appearing in (5) and (6) is actually a random variable. To show the robustness of our length regulation mechanism against random fluctuations in $\tau$, we assume a Gaussian distribution about the mean value $\tau_0$ with standard deviation $\sigma = 0.1\tau_0$ and solve Eqs. (2), (5), (6), and (10) for the axon dynamics. Figure S2 (left panel) shows that the axon reaches a stationary length that is almost identical to the stationary length for the case of a fixed $\tau$. The

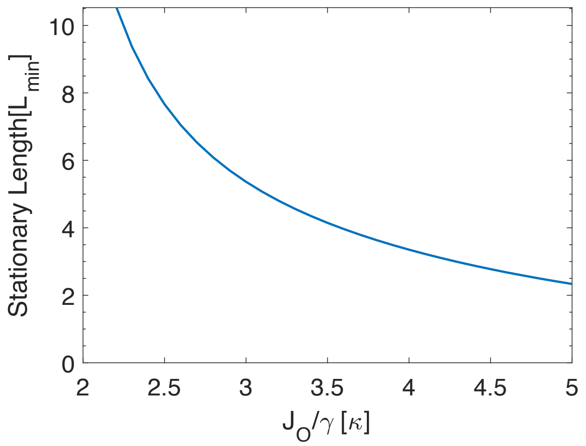


FIG. S1. (color online) Stationary axon length as a function of the coupling parameter $J_O$. Changes in $J_O$ correspond to changes in the concentration of dynein motors that transport the signal $O$ from the growth cone to the soma. The results are in agreement with experimental findings in the case of dynein depletion [20]. Parameter values are $J_R = 26 \times 10^{-5}\ \mu\mathrm{m}^{-1}\mathrm{s}^{-1}$, $J_0 = J_I = 55 \times 10^{-5}\ \mu\mathrm{m}^{-1}\mathrm{s}^{-1}$, $\kappa = 2 \times 10^{-2}\ \mu\mathrm{m}^{-1}$, $\kappa_R = 5 \times 10^{-3}\ \mu\mathrm{m}^{-1}$, $\gamma = 10^{-2}\,\mathrm{s}^{-1}$, $v_g = 0.1\,\mu\mathrm{m}^2\mathrm{s}^{-1}$, $v_s = 0.5\,\mu\mathrm{m}^2\mathrm{s}^{-1}$ and $n = 4$.

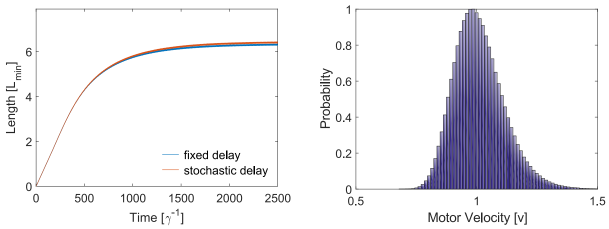


FIG. S2. (color online) Axon length dynamics for fixed and stochastic delay (left panel) and the corresponding velocity distribution for the stochastic case (right panel). In the stochastic dynamics we assumed that the delay time follows a Gaussian distribution with standard deviation $0.1\tau$ about the mean value $\tau$. The parameters are the same as the ones in Fig. 4.

corresponding velocity distribution is shown in the right panel.

## LOSSY TRANSPORT

In our analysis we assume that all the molecules leaving the soma get transported all the way to the growth cone and *vice versa*. In a real nerve cell, we might expect that some of them are lost as the motors transporting the molecules can detach and never make it to their destination. Assuming a loss rate $k_{\mathrm{loss}}$, the signal decays exponentially with a characteristic length $\lambda \equiv v/k_{\mathrm{loss}}$. The loss can thus be taken into account in the delay equations (5) and (6) of the main text by adding exponential factors:

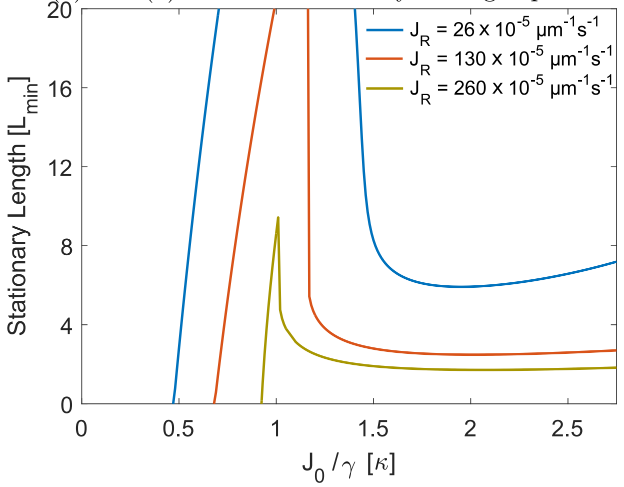


FIG. S3. (color online) Dependence of the mean length on $J_0$ for different values of the coupling constant $J_R$ and $J_I = J_0$ as given by the dynamic system with Eqs. (5) and (6) of the main text being replaced by Eqs. (S14) and (S15). We used a characteristic length of $\lambda = 1000\,\mu\mathrm{m}$. The other parameters are the same as in Fig. 4. $L_{\mathrm{min}}$ is calculated from Eq. (7) with $J_I = 55 \times 10^{-5}\ \mu\mathrm{m}^{-1}\mathrm{s}^{-1}$.

$$\dot{c}_I(t) = \left(J_0 - J_I f_\kappa\left(c_O(t-\tau)\right)\right)\exp\left(-L(t)/\lambda\right) - \gamma_I c_I(t) \tag{S14}$$

$$\dot{c}_O(t) = J_O f_\kappa\left(c_I(t-\tau)\right)\exp\left(-L(t-\tau)/\lambda\right) - \gamma_O c_O(t). \tag{S15}$$

As the signal $I$ is located at the growth cone, the length that has to be taken in the exponential is the current length. For the signal $O$, which acts at the soma, it has to be the length, when it left the growth cone, so $L$ at time $t - \tau$. With these modifications, the dynamics of the system does not change qualitatively. In particular, the stationary length still is a non-monotonic function of the base rate $J_0$ at which motors enter the axon, Fig. S3.
